# Supplementary material for: From curves to currents
Source: arXiv:2004.01550 source file (2024-12-09)

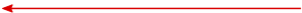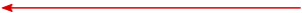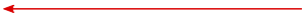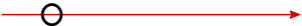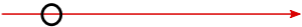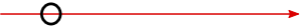

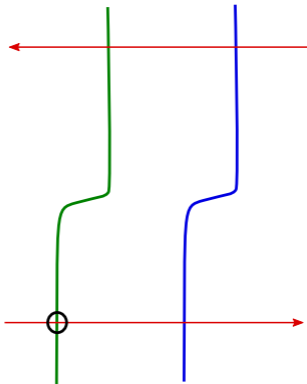

Supplement: Supplementary file 1 [file sm1.pdf]
