# Supplementary material for: From curves to currents
Source: arXiv:2004.01550 source file (2024-12-09)

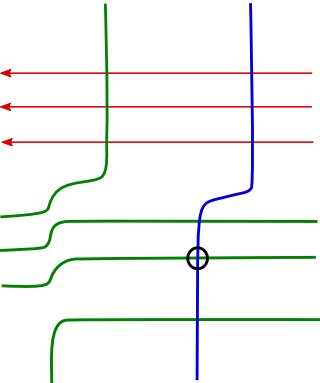

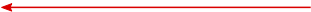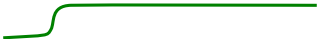

Supplement: Supplementary file 2 [file sm2.pdf]
